# Supplementary material for: Comprehensive language-image pre-training for 3D medical image understanding
Source: arXiv:2510.15042 source file (2026-08-15)
Supplement: Supplementary file 1 [file sentence_shortening_neg_llm.tex]

% \begin{table*}[]
%     \centering
% \begin{tabular}{l|ccc|cc|cc|cc}
% \toprule
% Eval & \multicolumn{3}{r}{Retrieval} & \multicolumn{2}{r}{Lin. Probe} & \multicolumn{2}{r}{Zero-shot (A)} & \multicolumn{2}{r}{Zero-shot (S)} \\
% Metric & R1 & R5 & R10 & AUPRC & AUROC & AUPRC & AUROC & AUPRC & AUROC \\
% \midrule
% Default & 8.27 & 22.64 & 31.66 & 55.41 & 83.11 & 43.48 & 76.48 & 34.77 & 66.91 \\
% Short sent. LLM & 2.59 & 9.28 & 16.05 & 50.78 & 80.94 & 44.33 & 78.06 & 33.16 & 67.84 \\
% Short sent. LLM p25 & 2.84 & 11.29 & 17.64 & 51.11 & 81.25 & 44.72 & 76.95 & 33.98 & 64.68 \\
% Short sent. LLM p25 neg & 2.01 & 9.62 & 18.48 & 52.32 & 81.94 & 43.67 & 78.05 & 41.59 & 72.91 \\
% Short sent. LLM p50 & 4.01 & 15.72 & 24.25 & 55.03 & 83.01 & 47.49 & 78.82 & 31.78 & 62.58 \\
% Short sent. LLM p75 & 4.93 & 16.89 & 25.59 & 54.81 & 83.14 & 47.58 & 78.27 & 31.42 & 66.68 \\
% \bottomrule
% \end{tabular}


%     \caption{Short sentence augmentation through an LLM. *neg indicates using short sentences denoted as negative as well.}
%     \label{tab:placeholder}
% \end{table*}

\begin{tabular}{l|ccc|cc|cc|cc}
\toprule
Eval & \multicolumn{3}{c}{Retrieval} & \multicolumn{2}{c}{Probing} & \multicolumn{2}{c}{Zero-shot (N)} & \multicolumn{2}{c}{Zero-shot (S)} \\
Metric & R1 & R5 & R10 & AUPRC & AUROC & AUPRC & AUROC & AUPRC & AUROC \\\midrule
\rowcolor{gray!20} Default & 8.27 & 22.64 & 31.66 & 55.41 & 83.11 & 43.48 & 76.48 & 34.77 & 66.91 \\\midrule
p=[10\%] & 12.71 & 29.01 & 39.30 & 56.91 & 83.76 & 45.81 & 77.93 & 39.55 & 71.15 \\
p=[25\%] & 11.54 & 27.68 & 38.04 & 56.45 & 83.87 & 47.12 & 78.67 & 35.13 & 68.10 \\
p=[50\%] & 11.20 & 28.01 & 38.21 & 56.32 & 83.91 & 46.07 & 78.63 & 37.09 & 70.24 \\
p=[75\%] & 9.78 & 25.92 & 34.36 & 56.97 & 84.01 & 46.41 & 78.74 & 34.70 & 68.19 \\
\bottomrule
\end{tabular}
